# Supplementary material for: Forecasting Time-to-Collision from Monocular Video: Feasibility, Dataset, and Challenges
Source: arXiv:1903.09102 source file (2020-11-02)
Supplement: Supplementary file 1 [file appendix.tex]

Here we report our initial experiments where we formulated the task of predicting near-collision time as a classification model. 

\subsection{Binary Classification: What happens 1 second into the future?}

In initial experimentation, we formulated the task as binary classification whether there is a near-collision in next one second or not. The output layer in Fig. \ref{fig:model} is replaced by a two-neuron layer followed by softmax function. The binary cross entropy loss is used to train the network. An alternative naive way to solve this task is to compare the foot of pedestrians' bounding boxes with a predefined threshold on pixel's vertical coordinate. The table \ref{tab:binary_classification} compares the F1 score from our learning approach versus the naive baseline. For the naive baseline, if the foot of the pedestrian lies in the lower $37.5\%$ (empirically found to be best) of the vertical size of image, we classify it as collision within one second.  

We use GradCAM \cite{gradCAM} to see which part of the image our trained network attends to. It first computes the gradient of the score for a class $c$ with respect to the feature maps of last convolutional layer. The gradients are global-average-pooled to get the importance of a feature map $k$ for class $c$. A weighted combination of forward activation maps is finally upsampled to the  size of input image to visualize the attention map. The confusion matrix over a test set passed through the trained network is reported in table \ref{tab:confusion_matrix}. To tackle the data imbalance between the collision instances (2106) and no collision instances (8579), a weighted sampler is used in training with collision instances having a weight of $0.6$ and no collision instances having a lower weight of $0.4$.
%% I should balance the training! 

    \begin{figure}[ht]
      \centering
      \includegraphics[height=7cm, width=\columnwidth]{figs/grad_binary_class.png}
      \caption{Visualization of heatmaps using GradCAM; Top Left: Two Persons going away, Top Right: One person with two probable trajectories, Bottom Left: A person going away, Bottom Right: A person approaching}
      \label{fig:gradcam1}
  \end{figure}

    \begin{figure}[ht]
      \centering
      \includegraphics[height=7cm, width=\columnwidth]{figs/gradCAM.pdf}
      \caption{Left: RGB Image, Right: Corresponding GradCAM}
      \label{fig:gradcam2}
  \end{figure}

\begin{table}[h]
\caption{Confusion Matrix from Binary Classification}\label{tab:confusion_matrix}
\noindent

\setlength\tabcolsep{0pt}
\begin{tabular}{c >{\bfseries}r @{\hspace{0.7em}}c @{\hspace{0.4em}}c @{\hspace{0.7em}}l}
  \multirow{10}{*}{\parbox{1.1cm}{\bfseries\raggedleft Actual\\ value}} & 
    & \multicolumn{2}{c}{\bfseries Prediction outcome} & \\
  & & \bfseries \small{collision} & \bfseries \small{no collision} \\
  & \small{collision} & \MyBox{634}{} & \MyBox{36}{} \\[2.4em]
  & \small{no collision} & \MyBox{53}{} & \MyBox{2840}{}  
\end{tabular}
\end{table}

\begin{table}[h]
\caption {Near-Collision Prediction formulated as Binary Classification: F1 Scores from our approach compared with a naive baseline} \label{tab:binary_classification} 
\begin{tabular}{|P{4cm}|P{2cm}|} \hline
Method  &  F1 Score \\ \hline
Naive baseline $(0.625 Y)$ & 0.8488 \\ \hline 
N-stream VGG $(N = 4)$ &  \textbf{0.9344} \\ \hline %% From slides  
\end{tabular}
\end{table}

\subsection{Multi-label Classification}
On previous task of binary classification for 0-1 sec, our deep learning approach performs better than the naive thresholding as reported in table \ref{tab:binary_classification}. We thus move on to increasing the difficulty of the task, i.e, a multi-label classification problem where we classify if there is going to be a near-collision instance in (1) within a second, (2) between 1-2 seconds, (2) between 2-3 seconds and/or (4) after 3 seconds. Our training and test data distribution for this multi-label classfication is provided in table \ref{tab:class_distribution}. For training, we used multilabel soft margin loss \cite{pytorch} as the loss function. The F1 scores reported in table \ref{tab:multi_label_classification} indicates that the naive baseline can give better predictions within 2 seconds into the future while the proposed multilabel deep neural network performs better for the latter classes, i.e., predictions in the range 2-3 seconds and after 3 seconds. One of the challenges of this multi-label formulation over the regression formulation is that we have to empirically decide a threshold on the confidence score for each class to classify it as the positive or negative label. The precision-recall curve or area under ROC curve \cite{roc} can be used to evaluate the performance of the trained model at different thresholds and then decide a threshold accordingly. \\

\begin{table}[h]
\caption {Class Distribution} \label{tab:class_distribution} 
\begin{tabular}{|P{2cm}|P{2cm}|P{2cm}|} \hline
Near-Collision Time  &  Training Data & Test Data \\ \hline
0-1 s &  4150 & 287 \\ \hline 
1-2 s &  2590 & 185 \\ \hline
2-3 s &  2185 & 169 \\ \hline
After 3 s & 13049  & 507 \\ \hline 
\end{tabular}
\end{table}

\begin{table}[h]
\caption {Near-Collision Prediction formulated as Multi-Class Classification} \label{tab:multi_label_classification} 
\begin{tabular}{|P{2cm}|P{2cm}|P{1.5cm}|P{1.5cm}|} \hline
Near-Collision Time  &  Vertical Image Coordinate for naive baseline $Y = 720$  & F1 Score from Naive Baseline & F1 Score from N-Stream VGG \\ \hline
0-1 s & $> 0.625Y$ &  0.849 & 0.759 \\ \hline 
1-2 s & $> 0.560Y$ & 0.720 & 0.630 \\ \hline
2-3 s & $> 0.520Y$ & \textbf{0.629} & \textbf{0.947} \\ \hline
After 3 s & $\le 0.520Y$ & \textbf{0.522}  & \textbf{0.620} \\ \hline 
\end{tabular}
\end{table}
